# Supplementary material for: Nonlocal Transport of Heat in Equilibrium Drift-Diffusion Systems
Source: arXiv:2207.01676 source file (2022-12-14)
Supplement: Supplementary file 1 [file supplementals.tex]

\begin{center}
	{\large
		{\bf
			Supplemental Materials for the manuscript \\ \vspace{0.25cm}
		}
	``\mytitle" \\ \vspace{0.25cm}
	}
	by F. St{\"a}bler and E. Sukhorukov
\end{center}

\section{Cross-capacitive coupling - Hamiltonian system}

Imagine an edge state, subdivided into mesocopic capacitors. Each capacitor consists of a piece of the edge state of length L and the interaction of the edge state is long range Coulombic, with self capacitance $C$. Furthermore assume, that the mesoscopic capacitors are interacting with their nearest neighbors via a cross capacitive ineraction of strength $C_X$. The distance between the capacitors is denoted by $W$. The Hamiltonian of inside a single capacitor at position $j$ looks like

\begin{equation}
    \mathcal{H}_j=\frac{\hbar v_F}{4\pi}  \int d{x} \left( \partial_x \phi_{ j}(x,t) \right)^2 + \frac{Q^2_j(t)}{2 C} + \frac{Q_j(t) Q_{j-1}(t)}{C_X}.
\end{equation}

The time evolution of the $\phi_{j}$ fields are given by
\begin{gather*}
    \partial_t \phi_{ j}(x,t) + v_F \partial_x \phi_{ j} (x,t) = -\frac{i}{\hbar} \left[\phi_{ j}(x,t),\frac{Q^2_{j'}(t)}{2 C} + \frac{Q_{j'-1}(t) Q_{j'}(t)}{C_X}\right],\\
  - \frac{i}{\hbar} \left[\phi_{ j} (x,t),\frac{Q^2_{j'}(t)}{2 C}\right] = -\frac{i e}{\hbar C} Q_{j'}(t)  \int \frac{d{y}}{2\pi} \left[\phi_{ j}(x,t),\partial_y \phi_{ j'}(y,t) \right]  = - \frac{e}{\hbar C} Q_j(t),\\
   - \frac{i}{\hbar} \left[\phi_{ j} (x,t),\frac{Q_{j'-1}(t) Q_{j'}(t)}{C_X}\right]\\= -\frac{i e}{\hbar C_X}  \int \frac{d{y}}{2\pi}  Q_{j'}(t) \left[\phi_{ j}(x,t),\partial_y \phi_{ j'-1}(y,t) \right]+ Q_{j'-1}(t) \left[\phi_{ j}(x,t),\partial_y \phi_{j'}(y,t) \right] \\=  -\frac{ e}{\hbar C_X} \left( Q_{j-1}(t) + Q_{j+1}(t) \right),
\end{gather*} where we used the commutation relation  $    \left[\phi_{ j}(x,t),\partial_y \phi_{ j'}(y,t) \right]=-2\pi i \delta(x-y) \delta_{j j'}.$ The full equation of motion are given by

\begin{equation}
     \partial_t \phi_{ j}(x,t) + v_F \partial_x \phi_{ j} (x,t) = - \frac{e}{\hbar C} \mathcal{Q}_j(t), \quad \mathcal{Q}_j(t)= Q_j(t) + \lambda \left( Q_{j-1}(t) + Q_{j+1}(t) \right), \quad \lambda = \frac{C}{C_X}.
\end{equation}

The solution of the equation of motion can be written as follows in frequency representation.

\begin{multline}
    \phi_{ j}(x,\omega) = \tilde{\phi}_{ j}(\omega) e^{\frac{i \omega  x}{v_F}} + \frac{ e}{i\omega \hbar C} \left( 1-e^{\frac{i \omega  x}{v_F}}\right) \mathcal{Q}_j(\omega) \\ = \tilde{\phi}_{ j}(0,\omega)(\omega) e^{\frac{i \omega  x}{v_F}} + \frac{1-e^{\frac{i \omega  x}{v_F}} }{i \omega \tau_{RC} } \left[\tilde{\phi}_{ j}(L,\omega) + \lambda\left(\tilde{\phi}_{ j-1}(L,\omega)+\tilde{\phi}_{ j+1}(L,\omega)\right) - L \leftrightarrow 0\right],
\end{multline} where $\tau_{RC}=R_Q C$ is the RC-time of the nodes and $\tilde{\phi}$ are the constants of integration. By taking a time derivative and multiplying both sides with the proper coefficients this translates into a formula for the currents inside the ohmic contact. In the following we  assume that we have only two nodes. The current incident to node $1$ is an equilibrium current $j_{0}(\omega)$ from a big reservoir at a zero potential and constant temperature. We can solve the system of equations for the outgoing currents as a function of the boundary current. We solve the following system of equations for $j_{\text{out}1}(\omega)$ and $j_{\text{out}2}(\omega)$

\begin{gather}
    j_{\text{out}1}(\omega) = j_{0}(\omega) e^{\frac{i \omega  L}{v_F}} + \frac{1-e^{\frac{i \omega  L}{v_F}} }{i \omega \tau_{RC} }\left[j_{\text{out}1}(\omega)-j_{0}(\omega) + \lambda\left(j_{\text{out}2}(\omega)-j_{\text{in}2}(\omega)\right)\right]\\
    j_{\text{out}2}(\omega) = j_{\text{in}2}(\omega) e^{\frac{i \omega  L}{v_F}} + \frac{1-e^{\frac{i \omega  L}{v_F}} }{i \omega \tau_{RC} }\left[j_{\text{out}2}(\omega)-j_{\text{in}2}(\omega)+ \lambda\left(j_{\text{out}1}(\omega)-j_{0}(\omega)\right)\right],
\end{gather} with the additional constraint of retardation $j_{\text{in}2}(\omega)= j_{\text{out}1}(\omega) e^{\frac{i \omega W}{v_F}}$. This gives

\begin{multline*}
    j_{\text{out}1}(\omega)  = \frac{j_0(\omega)}{D(\omega)} \left[4(1- \lambda ^2) \sin^2 \left(\frac{ \omega L }{2v_F}\right)  +2  \omega \tau_{RC}  \sin \left(\frac{ \omega L}{v_F}\right) +  \omega^2 \tau_{RC}^2\right],\\
    j_{\text{out}2}(\omega)
    =\frac{j_0(\omega)}{D(\omega)} \left[e^{\frac{i \omega  W}{v_F}} \left(4 \left(1-\lambda ^2-i \lambda  \omega  \tau_{RC}  e^{-\frac{i \omega  W}{v_F}}\right) \sin ^2\left(\frac{\omega  L}{2 v_F}\right)+2 i \omega 
   \tau_{RC}  \left(1-e^{\frac{i \omega  L}{v_F}}\right)+e^{\frac{i \omega  L}{v_F}} \omega ^2 \tau_{RC}^2\right) \right],\\
   D(\omega)=4 \left(1-\lambda ^2-i \tau_{RC}  \omega \right) \sin ^2\left(\frac{\omega  L}{2 v_F}\right)+\omega  \tau_{RC}   \left(2 \sin \left(\frac{\omega  L}{v_F}\right)+4 i \lambda  \sin ^2\left(\frac{\omega  L}{2 v_F}\right) e^{\frac{i
   \omega  W}{v_F}} \right) + \omega ^2  \tau_{RC} ^2 e^{-\frac{i L \omega }{v_F}}.
\end{multline*} We can see that the whole scattering matrix is unitary as it should be for a Hamiltonian system from the fact that $\left\langle j_{\text{out}2}(\omega) j_{\text{out}2}(-\omega) \right\rangle=\left\langle j_{0}(\omega) j_{0}(-\omega) \right\rangle$. However this is in general not true for the intermediate current $\left\langle j_{\text{out}1}(\omega) j_{\text{out}1}(-\omega) \right\rangle \neq\left\langle j_{0}(\omega) j_{0}(-\omega) \right\rangle$, because part of the heat is passed by the collective mode through the cross capacitive coupling. We will analyze the heat current corresponding to the intermediate current in different limits of $W$ and $L$.

\subsection{Limit of $W \rightarrow \infty$} 

This limit corresponds to the case where the distance between the nodes is very large. The phase factors $e^{\frac{i \omega  W}{v_F}}$ become fast oscillating functions and we average over these oscillations separately. We map the average integration onto the unit circle contour with $z\rightarrow e^{\frac{i \omega  W}{v_F}} $ and integrate over z. This gives

\begin{equation}
    \oint_C \frac{dz}{2\pi} S_1(\omega) \frac{|Y|^2}{\left(X+4 i \lambda \omega \tau_{RC} \sin^2 \left(\frac{ \omega L }{2v_F}\right) z\right)\left(X^*-4 i \lambda \omega \tau_{RC} \sin^2 \left(\frac{ \omega L }{2v_F}\right) \frac{1}{z}\right)} =S_1(\omega),
\end{equation} with 
\begin{gather}
    X(\omega)= 4 \left(1-\lambda ^2-i \tau_{RC}  \omega \right) \sin ^2\left(\frac{\omega  L}{2 v_F}\right)+2 \omega  \tau_{RC}  \sin \left(\frac{\omega  L}{v_F}\right) + \omega ^2  \tau_{RC} ^2 e^{-\frac{i L \omega }{v_F}}\\
    Y(\omega)=\left(4(1- \lambda ^2) \sin^2 \left(\frac{ \omega L }{2v_F}\right)  +2  \omega \tau_{RC}  \sin \left(\frac{ \omega L}{v_F}\right) +  \omega^2 \tau_{RC}^2\right),
\end{gather} which has one pole inside the contour independent of the parameters at 

\begin{equation}z_0 = \frac{4 i \lambda  \omega \tau_{RC} \sin ^2\left(\frac{\omega  L}{2 v_F}\right)}{4 \left(1-\lambda ^2\right) \sin ^2\left(\frac{\omega  L}{2 v_F}\right)+4 i \omega  \tau_{RC}  \sin
   ^2\left(\frac{\omega  L}{2 v_F}\right)+\omega ^2 \tau_{RC}^2 \cos \left(\frac{\omega  L}{v_F}\right)+\omega  \tau_{RC}  (2+i \omega  \tau_{RC} ) \sin \left(\frac{\omega  L}{v_F}\right)}.
   \end{equation}
   
    Physically this means that the correlation between the charge fluctuations of the left and right node are lost if they are far apart and the heat flux quantization is restored also in between the nodes. In the following we will thus always consider the strongly coupled limit $W\rightarrow 0$

\subsection{ Limit of $L\rightarrow 0$}

In this limit one immediately obtains

\begin{equation}
    \left\langle j_{\text{out}1}(\omega) j_{\text{out}1}(-\omega) \right\rangle = \left\langle j_{0}(\omega) j_{0}(-\omega) \right\rangle.
\end{equation} This limit corresponds to the non-interacting limit, where no charge fluctuations are excited in the nodes and thus no energy can be transferred. 

\subsection{ Limit of $L\rightarrow \infty$}

This is the first non-trivial limit in which the nodes are assumed to be large. We take $W \rightarrow 0$ and again average over the fast fluctuations with  $z\rightarrow e^{\frac{i \omega  L}{v_F}} $

\begin{equation}
   \left\langle j_{\text{out}1}(\omega) j_{\text{out}1}(-\omega) \right\rangle= \oint_C \frac{dz}{2\pi} S_1(\omega) \frac{ \left((z-1)^2 \left(\lambda ^2-1\right)-i \left(z^2-1\right) \omega \tau_{RC} +z  \omega^2 \tau_{RC}^2\right)^2}{i z \left((z-1)^2 \left(\lambda ^2-1\right)-i (z-1)
   (2+(z-1) \lambda )\omega \tau_{RC} + \omega ^2 \tau_{RC}^2\right) (\text{h.c.})} ,
\end{equation} which has always three poles inside the contour independent of the parameters. 

\begin{gather}
    z_0=0,\\
    z_1=\frac{\lambda ^2-1+i \lambda    \omega \tau_{RC}}{(\lambda -1) (1+\lambda +i   \omega \tau_{RC} )+\sqrt{-\lambda   \omega ^2 \tau_{RC}^2 (\lambda +i   \omega \tau_{RC})}},\\
    z_2=\frac{(\lambda -1) (1+\lambda +i  \omega \tau_{RC} )+\sqrt{-\lambda   \omega ^2 \tau_{RC}^2 (\lambda +i   \omega \tau_{RC} )}}{\lambda ^2+i \lambda  \omega \tau_{RC} -(1+i   \omega \tau_{RC} )^2}.
\end{gather}

The integral evaluates to

\begin{multline}\label{eq:app:Sint1}
   \left\langle j_{\text{out}1}(\omega) j_{\text{out}1}(-\omega) \right\rangle=   \frac{\left(\lambda-1 ^2\right)^2+\left(2+\lambda ^2\right)  \omega ^2 \tau_{RC}^2+ \omega ^4 \tau_{RC}^4}{\left(\lambda ^2-1\right)^2+(2+\lambda  (3 \lambda -4 )) 
   \omega ^2 \tau_{RC}^2+ \omega ^4 \tau_{RC}^4}S_1(\omega)\\
   \approx S_1(\omega) \left(1+\frac{2 \lambda (2-\lambda )   }{\left(\lambda ^2-1\right)^2}  \omega ^2\tau_{RC}^2\right),
\end{multline} which always gives a value larger than a flux quantum of heat if the frequency integral is performed.

\subsection{Equivalence to the reservoir model}

We note that this result can also be obtained by considering dissipative reservoirs instead of a large energy conserving system. The dynamics inside of the reservoir is as follows. A current entering the reservoir will be dissipated and heats the Ohmic contact. This creates voltage fluctuations, a Langevin source, with the temperature according to the dissipated current. The equation of motion slightly change and the problem simplifies. For the $L\rightarrow \infty$ limit you can equivalently solve the following set of equations.

\begin{gather}
    \frac{d}{d t} Q_1(t) = j_{\text{in}1}(t) - j_{\text{out}1}(t),\\
     \frac{d}{d t} Q_2(t) = j_{\text{in}2}(t) - j_{\text{out}2}(t),\\
     j_{\text{out}1}(t)= \frac{1}{\tau_{RC}}\left( Q_1(t)+\lambda  Q_2(t)\right) + j^c_{\text{out}1}(t),\\
     j_{\text{out}2}(t)= \frac{1}{\tau_{RC}}\left( Q_2(t)+\lambda  Q_1(t)\right) + j^c_{\text{out}2}(t),\\
     j_{\text{in}2}(t)=j_{\text{out}1}(t),
\end{gather} where $j^c_{\text{out}1/2}(t)$ are Langevin sources with a noise power that has the same temperature as the incoming current $j_0$. Solving these equation gives the same result as \cref{eq:app:Sint1}. If we take the limit $\tau_{RC}\rightarrow 0$ \cref{eq:app:Sint1} we obtain again a heat flux quantum, which signifies that the additional correlations imposed on this intermediate current are no Coulomb blockade effect, but rather dynamic out of phase fluctuations of the potentials in the nodes, which has a back action effect on the current and leads to a negative heat drag effect.

\subsection{Limit of finite $L$}

If $L$ is kept finite, \cref{eq:app:Sint1} is modified to be

\begin{multline}\label{eq:app:Sint1finiteL}
   \left\langle j_{\text{out}1}(\omega) j_{\text{out}1}(-\omega) \right\rangle\\= \frac{\left(4 \left(1-\lambda ^2\right) \sin ^2\left(\frac{\omega  L}{2 v_F}\right)+ \omega ^2 \tau_{RC}^2+2  \omega \tau_{RC} \sin \left(\frac{ \omega L }{v_F}\right)\right)^2}{\left(4
   (1-\lambda ) (1+\lambda -i   \omega\tau_{RC} ) \sin ^2\left(\frac{ \omega L}{2 v_F}\right)+\omega \tau_{RC} (2-i   \omega \tau_{RC}) \sin \left(\frac{ \omega L }{v_F}\right)+
   \omega ^2 \tau_{RC}^2 \cos \left(\frac{ \omega L }{v_F}\right)\right)\left(\text{h.c.} \vphantom{\sin^2\left(\frac{X}{Y}\right)}\right)}S_1(\omega).
\end{multline}

Which has resonances, but the heat flux will always be equal or larger to quantum. {\color{red} Can this be explained similarly to the resonantor in the Cheianov paper?}

\section{QPC coupling - Reservoir model 2 nodes}

We solve the following equation of motion for two reservoirs with capacitance $C$ connected by a QPC with transparency $\mathcal{T}$. As an additional complication we have $M$ incoming and outgoing channels into each node besides the QPC. This gives 

\begin{gather}
    \frac{d}{d t} Q_1(t) =   j_{\text{in}1}(t) - j_{\text{out}1}(t)  - j_{\Omega \rightarrow R}(t)+ j_{ R \rightarrow \Omega}(t),\\
    \frac{d}{d t} Q_2(t) =  j_{\text{in}2}(t) - j_{\text{out}2}(t)-j_{\Omega \rightarrow L}(t)+ j_{ L \rightarrow \Omega}(t),\\
    j_{ R \rightarrow \Omega}(t)= \mathcal{T} j_{\Omega \rightarrow L}(t)+(1-\mathcal{T}) j_{\Omega \rightarrow R}(t)+j_Q^c(t),\\
    j_{ L \rightarrow \Omega}(t)= \mathcal{T} j_{\Omega \rightarrow R}(t)+(1-\mathcal{T}) j_{\Omega \rightarrow L}(t)-j_Q^c(t),\\
    j_{\Omega \rightarrow R} = \frac{1}{\tau_{RC}}Q_1(t) + j^c_{\Omega \rightarrow R}(t),\\
    j_{\Omega \rightarrow L} = \frac{1}{\tau_{RC}}Q_2(t) + j^c_{\Omega \rightarrow L}(t),\\
     j_{\text{out}1}(t)= \frac{1}{\tau_{RC}}Q_1(t) + j^c_{\text{out}1}(t),\\
     j_{\text{out}2}(t)= \frac{1}{\tau_{RC}} Q_2(t) + j^c_{\text{out}2}(t),\\
     j_{\text{in}2}(t)=j_{\text{out}1}(t),
\end{gather}

The intermediate outgoing current $j_{\text{out}1}(t) $ is given by 

\begin{equation}
    j_{\text{out}1}(\omega) = \sum_{\alpha \in M} \mathrm{T}^{\text{out}1}_\alpha(\omega) j^{(c)}_\alpha(\omega),
\end{equation}with $M=\{\text{in}1,\text{out}1,\text{out}2,\Omega \rightarrow L,\Omega \rightarrow R,Q\}$ and 

\begin{gather}
    \mathrm{T}^{\text{out}1}_0(\omega)=\frac{1-i   \omega \tau_{RC} }{\mathcal{T} (2 i   \omega\tau_{RC} -1)-(1-i  \omega \tau_{RC} )^2},\\
    \mathrm{T}^{\text{out}1}_{\text{in}1}(\omega) = - \mathrm{T}^{\text{out}1}_0(\omega) \left( 1 + \frac{\mathcal{T}}{1-i  \omega \tau_{RC}}\right),\\
    \mathrm{T}^{\text{out}1}_{\text{out}1}(\omega)=1+\mathrm{T}^{\text{out}1}_0(\omega),\\
    \mathrm{T}^{\text{out}1}_{\text{out}2}(\omega)=\mathrm{T}^{\text{out}1}_0(\omega)\left(  \frac{\mathcal{T}}{1-i  \omega \tau_{RC}}\right),\\
    \mathrm{T}^{\text{out}1}_{\Omega \rightarrow L}(\omega)=-\mathcal{T} \mathrm{T}^{\text{out}1}_0(\omega),\\
    \mathrm{T}^{\text{out}1}_{\Omega \rightarrow R}(\omega)=\mathcal{T} \mathrm{T}^{\text{out}1}_0(\omega),\\
    \mathrm{T}^{\text{out}1}_{Q}(\omega)=- \mathrm{T}^{\text{out}1}_0(\omega).
\end{gather} Using these equations, the current current correlation function is given by

\begin{equation}
    \left\langle j_{\text{out}1}(\omega)j_{\text{out}1}(-\omega) \right\rangle = 1+\frac{2 \mathcal{T} \left(1+\mathcal{T}- \omega ^2 \tau_{RC}^2\right)}{(1+\mathcal{T})^2+2 (1+\mathcal{T}) (1+2 \mathcal{T})\omega ^2 \tau_{RC}^2+ \omega ^4 \tau_{RC}^4},
\end{equation} which in the Coulomb Blockade regime ($\tau_{RC}\rightarrow0$) reduces to

\begin{equation}
    \left\langle j_{\text{out}1}(\omega)j_{\text{out}1}(-\omega) \right\rangle = 1+\frac{2 \mathcal{T}}{1+\mathcal{T}}.
\end{equation} The CB effect thus enhances the correlation of the intermediate current.

\section{Cross-capacitive coupling -  Transmission line}

We start from a TL, where every node is a infinte ohmic reservoir with capacitance $C$, connected with a chiral channel to the next reservoir. Furthermore, we introduce a capacitive cross coupling $C_x$ between the reservoirs.

\begin{figure}[htbp]
    \centering
    \includegraphics[width=\textwidth]{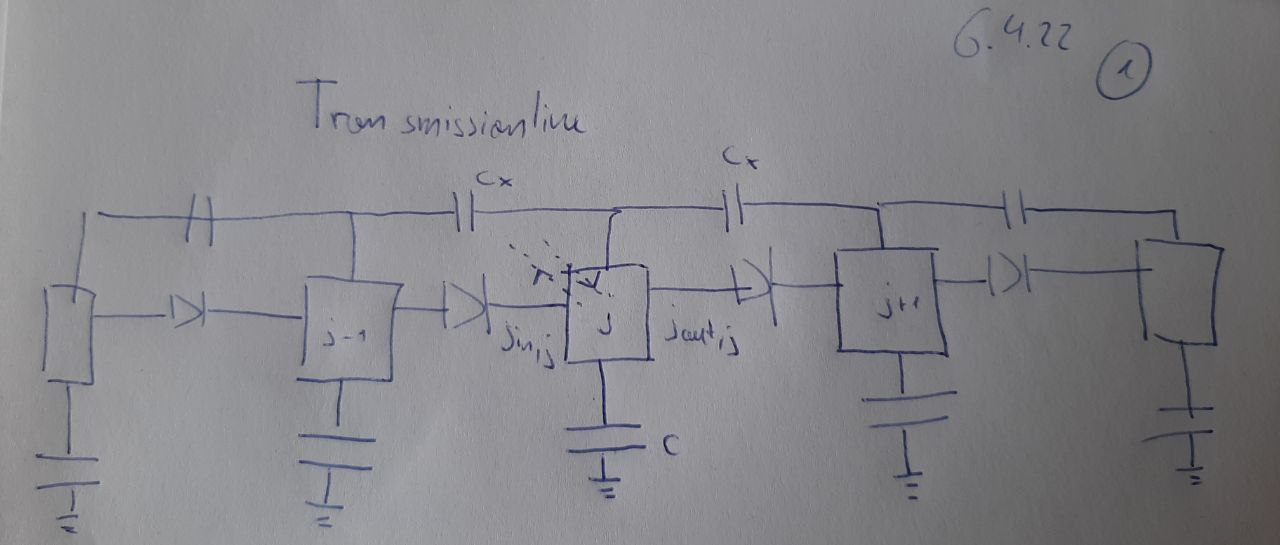}
    \label{fig:TLCx_draft}
\end{figure}

We derive the equation of motion from the Hamiltonian of within a single node at position $j$. Later we can see how to obtain this result in an easier way. The Hamiltonian is given by

\begin{equation}
    \mathcal{H}_j=\frac{\hbar v_F}{4\pi} \sum_\sigma \int d{x} \left( \partial_x \phi_{\sigma j}(x,t) \right)^2 + \frac{Q^2_j(t)}{2 C} + \frac{Q_j(t) Q_{j-1}(t)}{C_x}.
\end{equation}

The time evolution of the $\phi_{\sigma j}$ fields are given by
\begin{multline*}
   \sigma \partial_t \phi_{\sigma j}(x,t) + v_F \partial_x \phi_{\sigma j} (x,t) = -\frac{i}{\hbar} \left[\phi_{\sigma j}(x,t),\frac{Q^2_{j'}(t)}{2 C} + \frac{Q_{j'-1}(t) Q_{j'}(t)}{C_x}\right],\\
  - \frac{i}{\hbar} \left[\phi_{\sigma j} (x,t),\frac{Q^2_{j'}(t)}{2 C}\right] = -\frac{i e}{\hbar C} Q_{j'}(t) \sum_{\sigma'} \int \frac{d{y}}{2\pi} \left[\phi_{\sigma j}(x,t),\partial_y \phi_{\sigma' j'}(y,t) \right]  = - \frac{e}{\hbar C} Q_j(t),\\
   - \frac{i}{\hbar} \left[\phi_{\sigma j} (x,t),\frac{Q_{j'-1}(t) Q_{j'}(t)}{C_x}\right]\\= -\frac{i e}{\hbar C_x}  \sum_{\sigma'} \int \frac{d{y}}{2\pi}  Q_{j'}(t) \left[\phi_{\sigma j}(x,t),\partial_y \phi_{\sigma' j'-1}(y,t) \right]+ Q_{j'-1}(t) \left[\phi_{\sigma j}(x,t),\partial_y \phi_{\sigma' j'}(y,t) \right] \\=  -\frac{  e}{\hbar C_x} \left( Q_{j-1}(t) + Q_{j+1}(t) \right),
\end{multline*} where we used the commutation relation 

\begin{equation}
    \left[\phi_{\sigma j}(x,t),\partial_y \phi_{\sigma' j'}(y,t) \right]=-2\pi i \delta(x-y) \delta_{j j'} \delta_{\sigma \sigma'}.
\end{equation}

The full equation of motion are given by

\begin{equation}
    \sigma \partial_t \phi_{\sigma j}(x,t) + v_F \partial_x \phi_{\sigma j} (x,t) = - \frac{e}{\hbar C} \mathcal{Q}_j(t), \quad \mathcal{Q}_j(t)= Q_j(t) + \lambda \left( Q_{j-1}(t) + Q_{j+1}(t) \right), \quad \lambda = \frac{C}{C_x}.
\end{equation}

This equation can be solved going to the frequency representation, and the solution of the eom inside of the reservoir is exactly the same as in the ohmic contact paper. We find

\begin{equation}
    \phi_{\sigma j}(x,\omega) = \tilde{\phi}_{\sigma j}(\omega) e^{\frac{i \omega \sigma x}{v_F}} + \frac{\sigma e}{\hbar C} \frac{\mathcal{Q}_j(\omega)}{i\omega - \sigma \varepsilon} e^{\frac{\varepsilon x}{v_F}}.
\end{equation} We can further simplify this expression using the definition of $Q_j(t)=\sum_\sigma \int_{-\infty}^0 d{x} \ \rho_{\sigma j}(x) e^{\frac{\varepsilon x}{v_F}} = \sum_\sigma \tilde{\phi}_{\sigma j}(\omega) $ and find

\begin{equation}
    \phi_{\sigma j}(x,\omega) = \tilde{\phi}_{\sigma j}(\omega) e^{\frac{i \omega \sigma x}{v_F}} + \frac{\sigma }{R_q C}\sum_{\sigma'} \frac{\tilde{\phi}_{\sigma' j}(\omega) + \lambda\left(\tilde{\phi}_{\sigma j-1}(\omega)+\tilde{\phi}_{\sigma j+1}(\omega)\right)}{i\omega - \sigma \varepsilon} e^{\frac{\varepsilon x}{v_F}}.
\end{equation} Next, use a discrete Fourier transformation of the form

\begin{gather} 
	X_j(t)=\sum\limits_{k=0}^{N-1} \int \frac{d{\omega}}{2\pi} e^{i\frac{2 \pi k}{N} j-i\omega t} X_k(\omega),\\ 	X_k(\omega)=\frac{1}{N}\sum\limits_{j=0}^{N-1} \int d{t} \  e^{-i \frac{2 \pi k}{N}  j+i \omega t} X_j(t),
\end{gather} and take the large N limit 
\begin{equation*}
    \lim\limits_{N \rightarrow \infty}\frac{1}{N}\sum_{k=0}^{N-1} \rightarrow \int_{-\pi/\xi}^{\pi/\xi} \frac{d{k}}{2\pi},
\end{equation*} where we introduced the distance between the nodes $\xi$. We find in the limit $\varepsilon \rightarrow 0$

\begin{equation}
    \phi_{\sigma k}(x,\omega) = \tilde{\phi}_{\sigma k}(\omega) e^{\frac{i \omega \sigma x}{v_F}} + \frac{\sigma }{i\omega R_q C} \left(1 + 2\lambda \cos\left( k \xi \right)\right)\sum_{\sigma'} \tilde{\phi}_{\sigma' k}(\omega).
\end{equation} Next, we determine the constants of integration by matching the boundary conditions

\begin{align}
    \delta I_{c}(k,\omega) &\overset{!}{=}  \frac{i \omega e}{2\pi} \phi_{+,k} (-W,\omega), \\
    \Delta I_{\text{in}}(k,\omega) &\overset{!}{=}  \frac{-i \omega e}{2\pi} \phi_{-,k} (0,\omega), 
\end{align} from which we can find $\Delta I_{\text{out}}(k,\omega) \overset{!}{=} \frac{i \omega e}{2\pi} \phi_{+,k} (0,\omega)$ as a function of the currents above. We treat the coordinate $W$ as finite but large and neglect all fast oscillating terms proportional to that coordinate.

This gives us

\begin{gather}
    \Delta I_{\text{out}}(k,\omega) = T_c(k,\omega) \delta I_{c}(k,\omega) + T_{\text{in}}(k,\omega)\Delta I_{\text{in}}(k,\omega),\\  T_{\text{in}}(k,\omega)-1 = -T_c(k,\omega)=\frac{i \omega R_q C }{ 1-i \omega R_q C+2 \lambda  \cos \left(k \xi \right)}.
\end{gather} Note that $\left|T_c\right|^2+\left|T_{\text{in}}\right|^2=1$, reflecting the unitarity of the scattering matrix, however there can be out of phase oscillations of the potentials due to their non-local interaction. The same equations can can be obtained much easier by solving the following set of equations

\begin{gather}
    \frac{d{t}}Q_j(t)=\Delta I_{\text{in}} -\Delta I_{\text{out}},\\
    \Delta I_{\text{out}} = \frac{1}{R_q C} \mathcal{Q}_j(t) +  \delta I_{c, j}(t),
\end{gather} where the first equation implies charge conservation at each node and the second equation is a modified Langevin equation. We promote these equations to transmission line equations, by demanding that $ \Delta I_{\text{in},j}(\omega)=\Delta I_{\text{out},j-1}(\omega)$. After FT we solve for $\Delta I_{\text{out}}(k,\omega)$

\begin{equation}
  \Delta I_{\text{out}}(k,\omega) =   \frac{i \omega R_q C  }{i \omega R_q C+ \left(e^{-i k \xi }-1\right) \left(1+  2 \lambda   \cos (k \xi )\right)} \delta I_{c}(k,\omega)
\end{equation}

Since the system between the nodes is free chiral, we can obtain the HF by computing the outgoing current correlation function

\begin{multline}
  \left\langle \Delta I_{\text{out}}(k,\omega)\Delta I_{\text{out}}(-k,-\omega) \right\rangle = \\\frac{\omega^2 R_q^2 C^2}{\left[i \omega R_q C+ \left(e^{-i k \xi }-1\right) \left(1+  2 \lambda   \cos (k \xi )\right) \right]\left[-i \omega R_q C+ \left(e^{i k \xi }-1\right) \left(1+  2 \lambda   \cos (k \xi )\right) \right]}   S_c(\omega)
\end{multline}

We map this on $z$-space by the transformation $z=e^{i k \xi}$. That gives 

\begin{equation}
    -\frac{i \tau ^2 \omega ^2}{ \left((z-1) \left(1+ \lambda  \left(\frac{1}{z}+z\right) \right)-i \tau  \omega \right) \left(\left(1-z\right)
   \left(1+ \lambda  \left(\frac{1}{z}+z\right) \right)+i z \tau  \omega \right)}
\end{equation}

The integral over z on a circular contour has always three poles inside and three poles outside of the contour at any given time. Let us look at the simplified integral first

\begin{equation}
    -\frac{i \tau ^2 \omega ^2}{ \left((z-1) u[z] -i \tau  \omega \right) \left(\left(1-z\right)
   u[z] +i z \tau  \omega \right)}, 
\end{equation} with $u[z] = 1+ \lambda  \left(\frac{1}{z}+z\right)$. The integral for $u[z]=u_0$ has two poles

\begin{gather}
    z_1 = \frac{u_0}{u_0-i \omega \tau}, \\
    z_2 = \frac{u_0+i \omega \tau }{u_0}.
\end{gather} It can be easily seen, that independent of the value of $u_0$ the pole $z_1$ is always inside of the contour and is the desired pole close to $z=1$ for $\omega\rightarrow0$. We iterate $z_1$ around $z \rightarrow 1$ often enough, so that it's Taylor series does not change up to 4th order. We compute the residue around that point using that 

\begin{equation}
    \text{res}|_{z,z_0}\frac{1}{f(z)}=\frac{1}{f'(z_0)}.
\end{equation}

This gives the following frequency dependent function 

\begin{equation}
\left\langle \Delta I_{\text{out}}(k,\omega)\Delta I_{\text{out}}(-k,-\omega) \right\rangle = \frac{(1+2 \lambda )^3}{(1+2 \lambda )^3-2 \lambda  \tau ^2 \omega ^2}  S_c(\omega) + \text{other residues}.
\end{equation} We see that corrections to the HFQ start in the order $\omega^2$. To compute the corrections of the other poles we can thus assume $\omega=0$ in the denominator, which gives the desired correction. Picking up the remaining double pole leads to the following correction

\begin{equation}
\left\langle \Delta I_{\text{out}}(k,\omega)\Delta I_{\text{out}}(-k,-\omega) \right\rangle \approx \left( 1+\frac{2 \lambda  \tau ^2 \omega ^2}{(1+2 \lambda )^3}-\frac{2 (-1+\lambda ) \lambda  \tau ^2 \omega ^2}{(1-2 \lambda )^{3/2} (1+2 \lambda )^{5/2}}\right) S_c(\omega).
\end{equation}

{\color{red} Open questions:

\begin{itemize}
    \item How am I sure that I don't miss a $1/\omega^2$ contribution in the other poles.
    \item Is the energy that propagates elsewhere $\sim d/dt<Q_j Q_{j-1}>/C_x$?
\end{itemize}}

\section{QPC coupling - Transmission line}

We again start from a TL this time with resevoirs connected by a QPC and a chiral channel. The transmission probability is given by $\mathcal{T}$. The equation of motion including the noise produced by the QPC are

\begin{gather}
    -i \omega  \delta Q_k(\omega )=(e^{-i k \xi}-1)\Delta I_{out,k}(\omega)+\Delta I^{R\rightarrow\Omega}_{k}(\omega)- \Delta I^{\Omega\rightarrow R}_{k}(\omega)+I^{L\rightarrow\Omega}_{k}(\omega)-\Delta I^{\Omega\rightarrow L}_{k}(\omega),\\
    \Delta I_{out,k}(\omega)=\frac{1}{\tau} \delta Q_k(\omega )+\delta I_{out,k}(\omega),\\
    \Delta I^{\Omega\rightarrow L/R}_{k}(\omega)=\frac{1}{\tau} \delta Q_k(\omega )+\delta I^{\Omega\rightarrow L/R}_{k}(\omega),\\
    \Delta I^{R\rightarrow\Omega}_{k}(\omega)= \mathcal{T} e^{i k \xi } \Delta I^{\Omega\rightarrow L}_{k}(\omega) +\left(1-\mathcal{T}\right) \Delta I^{\Omega\rightarrow R}_{k}(\omega) + \delta I^Q_k(\omega),\\
    \Delta I^{L\rightarrow\Omega}_{k}(\omega)= \mathcal{T} e^{-i k \xi } \Delta I^{\Omega\rightarrow R}_{k}(\omega) +\left(1-\mathcal{T}\right) \Delta I^{\Omega\rightarrow L}_{k}(\omega) - e^{-i k \xi } \delta I^Q_k(\omega).
\end{gather}

We can solve these equations for the collective mode contribution in terms of the sources

\begin{equation}
    \delta Q_k(\omega) =  \frac{\left(e^{-i k\xi}-1\right) \tau  \left(-\delta I_{out,k}(\omega)+\delta I^Q_k(\omega)+e^{i k\xi} \mathcal{T} \delta I^{\Omega\rightarrow L}_{k}(\omega)-\mathcal{T} \delta I^{\Omega\rightarrow R}_{k}(\omega)\right)}{e^{-i k \xi}-1-2 \mathcal{T} (1-\cos (k \xi))+i \tau  \omega }.
\end{equation} We continue as follows. We compute the outgoing heat current in the chiral part of the system. The QPC noise power can be determined from energy balance, see the paper. We find three poles to be always inside. We pickup the poles and compute the residues exactly and expand the result in small $\omega$. This gives

\begin{equation}
   \left\langle \Delta I_{\text{out}}(k,\omega)\Delta I_{\text{out}}(-k,-\omega) \right\rangle= \int \frac{d k}{2\pi} \frac{2 \left(4 \mathcal{T}+8 \mathcal{T}^2\right) \sin ^2\left(\frac{k\xi}{2}\right)-4 \mathcal{T}^2 \sin ^2(k\xi)+\omega ^2 \tau ^2}{2-2 (1+2 \mathcal{T})^2 \cos (k\xi)+4 \left(\mathcal{T}+\mathcal{T}^2\right) \left(1+\cos
   ^2(k\xi)\right)-2 \omega  \tau  \sin (k\xi)+\omega ^2 \tau ^2},
\end{equation} where we have a dynamical component and a Coulomb blockade component given by

\begin{multline}
   \left\langle \Delta I_{\text{out}}(k,\omega)\Delta I_{\text{out}}(-k,-\omega) \right\rangle|_{\tau\rightarrow0}\\ =\int \frac{d k}{2\pi} \frac{2 \left(4 \mathcal{T}+8 \mathcal{T}^2\right) \sin ^2\left(\frac{k \xi}{2}\right)-4 \mathcal{T}^2 \sin ^2(k \xi)+\omega ^2 \tau ^2}{2-2 (1+2 \mathcal{T})^2 \cos (k\xi)+4 \left(\mathcal{T}+\mathcal{T}^2\right) \left(1+\cos
   ^2(k\xi)\right)-2 \omega  \tau  \sin (k\xi)+\omega ^2 \tau ^2}=\frac{2 \mathcal{T}}{1+\mathcal{T}},
\end{multline}

\begin{equation}
\left\langle \Delta I_{\text{out}}(k,\omega)\Delta I_{\text{out}}(-k,-\omega) \right\rangle \approx \left(1+\frac{2 \mathcal{T}}{1+\mathcal{T}}-6 \mathcal{T} \left(1 +2 \mathcal{T} \right) \tau ^2 \omega ^2\right) S_c(\omega),
\end{equation} where we find the surprising zero mode of heat, which is the exact $\omega=0$ part of the integral. This part was absent before, because the whole integral was $\sim \omega^2$. This is a result of an enhancement of correlations in the Coulomb blockade regime where $\tau\rightarrow0$.
